# Supplementary material for: 3DCoMPaT200: Language-Grounded Compositional Understanding of Parts and Materials of 3D Shapes
Source: arXiv:2501.06785 source file (2025-01-12)
Supplement: Supplementary file 1 [file appendix.tex]

\section{Appendix}
% \subsection{Data Creation}
% The data is collected through a collaboration with an industry partner to create and annotate the shapes. We provided a list of guidelines for each category and its associated fine parts segmentation. After the meshes are prepared, we go through an intensive verification of the labels and their suitable material assignation. In addition, we prepare the fine-to-coarse parts mapping and the suitable materials for the coarse-grained parts.
% each group of similar parts are assigned a common coarse part class that best describes it as shown in figure \ref{coarse_mapping}
% \begin{figure}[!h]
%     \centering
%     \includegraphics[width=\linewidth]{figs/semantics.pdf}
%     \caption{Illustrating Fine-grained to Coarse-grained mapping on a scooter shape} 
%     \label{coarse_mapping}
% \end{figure}

% \subsection{Qualitative Segmentation results}
% \begin{figure}[!h]
%     \centering
%     \includegraphics[width=\linewidth]{figs/tripod.pdf}
%     \caption{Qualitative segmentation results on a Tripod shape} 
%     \label{tripod}
% \end{figure}

% \begin{figure}[!h]
%     \centering
%     \includegraphics[width=\linewidth]{figs/lamplight.pdf}
%     \caption{Qualitative segmentation results on a LampLight shape} 
%     \label{lamplight}
% \end{figure}

% \begin{figure}[!h]
%     \centering
%     \includegraphics[width=\linewidth]{figs/mouse.pdf}
%     \caption{Qualitative segmentation results on a Mouse shape} 
%     \label{mouse}
% \end{figure}
